# Supplementary material for: Reference-Aware Language Models
Source: arXiv:1611.01628 source file (2017-08-09)
Supplement: Supplementary file 1 [file appendix.pdf]

## A Visualization

M: Hello , welcome to the Cambridge restaurant system ? You can ask for restaurants by area , price range or food type . How may I help you ?  
 U: and expensive restaurant that serves tuscan food  
 M: Sorry there is no tuscan restaurant in the expensive price range  
 U: french food  
 M: cote is a great restaurant serving french food and it is in the expensive price range  
 U: may i have the phone number  
 M: The phone number of cote is 01223 311053 .  
 U: thank you good bye

(a) Dialogue script

| NAME                    | PRICE RANGE | FOOD    | AREA   | ADDRESS                                                    | POST CODE    | PHONE        |
|-------------------------|-------------|---------|--------|------------------------------------------------------------|--------------|--------------|
| charlie chan            | cheap       | chinese | east   | Regent Street City Centre                                  | C.B 2, 1 D.B | 01223 361763 |
| chiquito restaurant bar | expensive   | mexican | south  | 2G Cambridge Leisure Park Cherry Hinton Road Cherry Hinton | C.B 1, 7 D.Y | 01223 400170 |
| city stop               | expensive   | food    | north  | Cambridge City Football Club Milton Road Chesterton        | .EMPTY       | 01223 363270 |
| clowns cafe             | expensive   | italian | centre | .EMPTY                                                     | C.B 1, 1 L.N | 01223 355711 |
| cocum                   | expensive   | indian  | west   | 71 Castle Street City Centre                               | C.B 3, 0 A.H | 01223 366668 |
| cote                    | expensive   | french  | centre | Bridge Street City Centre                                  | C.B 2, 1 U.F | 01223 311053 |
| curry garden            | expensive   | indian  | centre | 106 Regent Street City Centre                              | .EMPTY       | 01223 302330 |
| curry king              | expensive   | indian  | centre | 5 Jordans Yard Bridge Street City Centre                   | C.B 1, 2 B.D | 01223 324351 |
| curry prince            | moderate    | indian  | east   | 451 Newmarket Road Fen Ditton                              | C.B 5, 8 J.J | 01223 566388 |

(b) Attention heat map: cote is a great restaurant serving french food and it is in the expensive price range.

| NAME                    | PRICE RANGE | FOOD    | AREA   | ADDRESS                                                    | POST CODE    | PHONE        |
|-------------------------|-------------|---------|--------|------------------------------------------------------------|--------------|--------------|
| charlie chan            | cheap       | chinese | east   | Regent Street City Centre                                  | C.B 2, 1 D.B | 01223 361763 |
| chiquito restaurant bar | expensive   | mexican | south  | 2G Cambridge Leisure Park Cherry Hinton Road Cherry Hinton | C.B 1, 7 D.Y | 01223 400170 |
| city stop               | expensive   | food    | north  | Cambridge City Football Club Milton Road Chesterton        | .EMPTY       | 01223 363270 |
| clowns cafe             | expensive   | italian | centre | .EMPTY                                                     | C.B 1, 1 L.N | 01223 355711 |
| cocum                   | expensive   | indian  | west   | 71 Castle Street City Centre                               | C.B 3, 0 A.H | 01223 366668 |
| cote                    | expensive   | french  | centre | Bridge Street City Centre                                  | C.B 2, 1 U.F | 01223 311053 |
| curry garden            | expensive   | indian  | centre | 106 Regent Street City Centre                              | .EMPTY       | 01223 302330 |
| curry king              | expensive   | indian  | centre | 5 Jordans Yard Bridge Street City Centre                   | C.B 1, 2 B.D | 01223 324351 |
| curry prince            | moderate    | indian  | east   | 451 Newmarket Road Fen Ditton                              | C.B 5, 8 J.J | 01223 566388 |

(c) Attention heap map: The phone number of cote is 01223 311053 .

Table 7: Dialogue visualization 1

M: Hello , welcome to the Cambridge restaurant system ? You can ask for restaurants by area , price range or food type . How may I help you ?  
 U: cheap restaurant  
 M: What kind of food would you like ?  
 U: in the west part of town  
 M: la margherita is a nice restaurant in the west of town in the cheap price range  
 U: address  
 M: Sure , la margherita is on 15 Magdalene Street City Centre  
 U: thank you  
 M: la margherita is a nice restaurant in the west of town in the cheap price range  
 U: good bye

(a) Dialogue script

| NAME               | PRICE RANGE | FOOD          | AREA   | ADDRESS                         | POST CODE    | PHONE        |
|--------------------|-------------|---------------|--------|---------------------------------|--------------|--------------|
| india house        | expensive   | indian        | west   | 31 Newnham Road Newnham         | _EMPTY       | 01223 461661 |
| j restaurant       | cheap       | oriental      | centre | 86 Regent Street City Centre    | C.B 2, 1 D.P | 01223 307581 |
| jinling noodle bar | moderate    | chinese       | centre | 11 Peas Hill City Centre        | C.B 2, 3 P.P | 01223 566188 |
| kohinoor           | cheap       | indian        | centre | 74 Mill Road City Centre        | _EMPTY       | 01223 323639 |
| kymmoy             | expensive   | oriental      | centre | 52 Mill Road City Centre        | C.B 1, 2 A.S | 01223 311911 |
| la margherita      | cheap       | italian       | west   | 15 Magdalene Street City Centre | C.B 3, 0 A.F | 01223 315232 |
| la mimosa          | expensive   | mediterranean | centre | Thompsons Lane Fen Ditton       | C.B 5, 8 A.Q | 01223 362525 |
| la raza            | cheap       | spanish       | centre | 4 - 6 Rose Crescent             | C.B 2, 3 L.L | 01223 464550 |
| la tasca           | moderate    | spanish       | centre | 14 -16 Bridge Street            | C.B 2, 1 U.F | 01223 464630 |
| lan hong house     | moderate    | chinese       | centre | 12 Norfolk Street City Centre   | _EMPTY       | 01223 350420 |

(b) Attention heat map: la margherita is a nice restaurant in the west of town in the cheap price range

| NAME               | PRICE RANGE | FOOD          | AREA   | ADDRESS                         | POST CODE    | PHONE        |
|--------------------|-------------|---------------|--------|---------------------------------|--------------|--------------|
| india house        | expensive   | indian        | west   | 31 Newnham Road Newnham         | _EMPTY       | 01223 461661 |
| j restaurant       | cheap       | oriental      | centre | 86 Regent Street City Centre    | C.B 2, 1 D.P | 01223 307581 |
| jinling noodle bar | moderate    | chinese       | centre | 11 Peas Hill City Centre        | C.B 2, 3 P.P | 01223 566188 |
| kohinoor           | cheap       | indian        | centre | 74 Mill Road City Centre        | _EMPTY       | 01223 323639 |
| kymmoy             | expensive   | oriental      | centre | 52 Mill Road City Centre        | C.B 1, 2 A.S | 01223 311911 |
| la margherita      | cheap       | italian       | west   | 15 Magdalene Street City Centre | C.B 3, 0 A.F | 01223 315232 |
| la mimosa          | expensive   | mediterranean | centre | Thompsons Lane Fen Ditton       | C.B 5, 8 A.Q | 01223 362525 |
| la raza            | cheap       | spanish       | centre | 4 - 6 Rose Crescent             | C.B 2, 3 L.L | 01223 464550 |
| la tasca           | moderate    | spanish       | centre | 14 -16 Bridge Street            | C.B 2, 1 U.F | 01223 464630 |
| lan hong house     | moderate    | chinese       | centre | 12 Norfolk Street City Centre   | _EMPTY       | 01223 350420 |

(c) Attention heap map: Sure , la margherita is on 15 Magdalene Street City Centre.

Table 8: Dialogue visualization 2

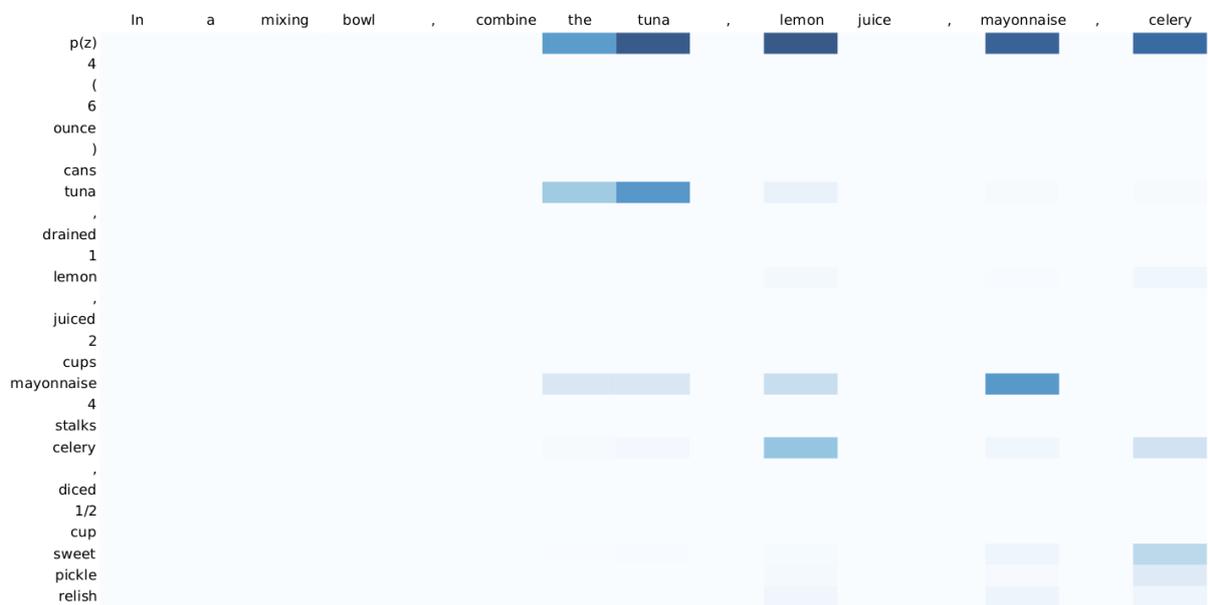

(a) part 1

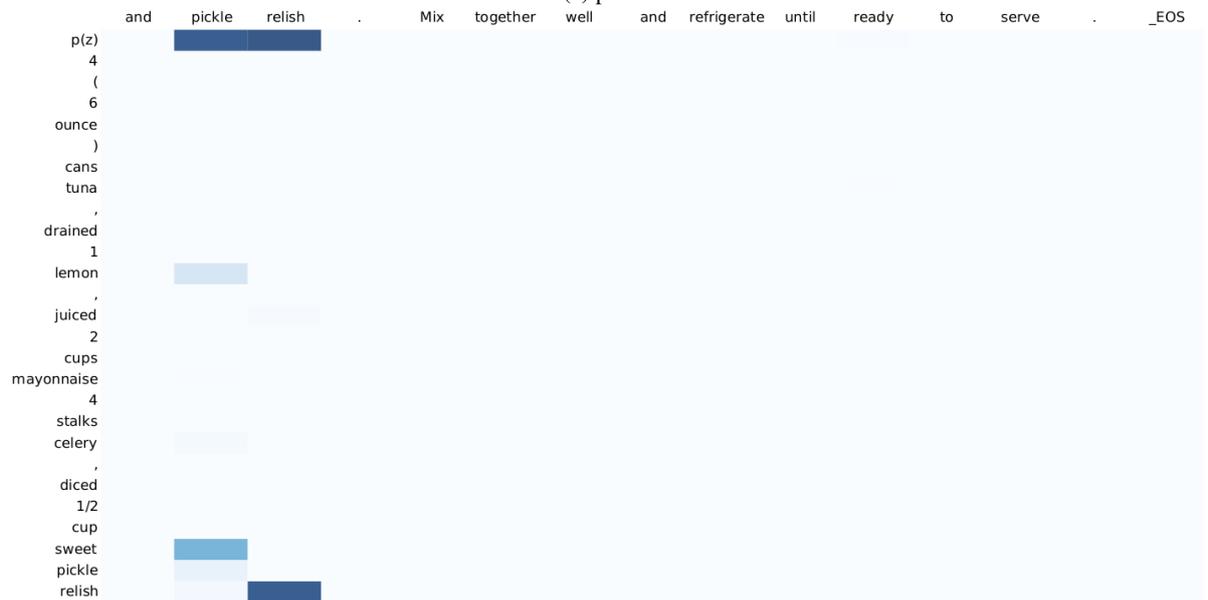

(b) part 2

Figure 6: Recipe heat map example 1. The ingredient tokens appear on the left while the recipe tokens appear on the top. The first row is the  $p(z_v|s_v)$ .

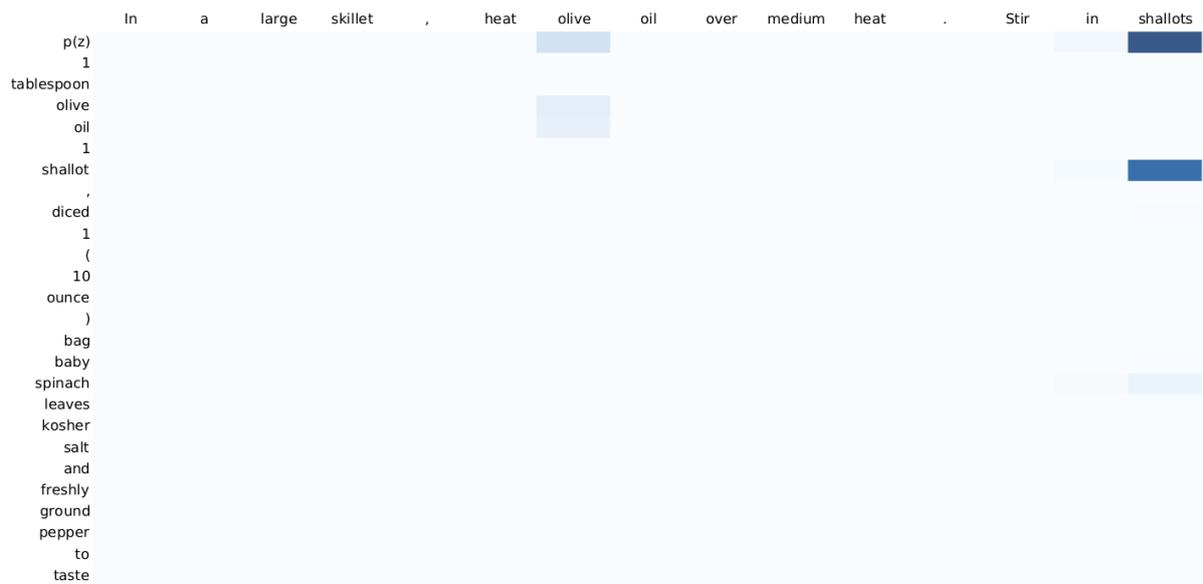

(a) part 1

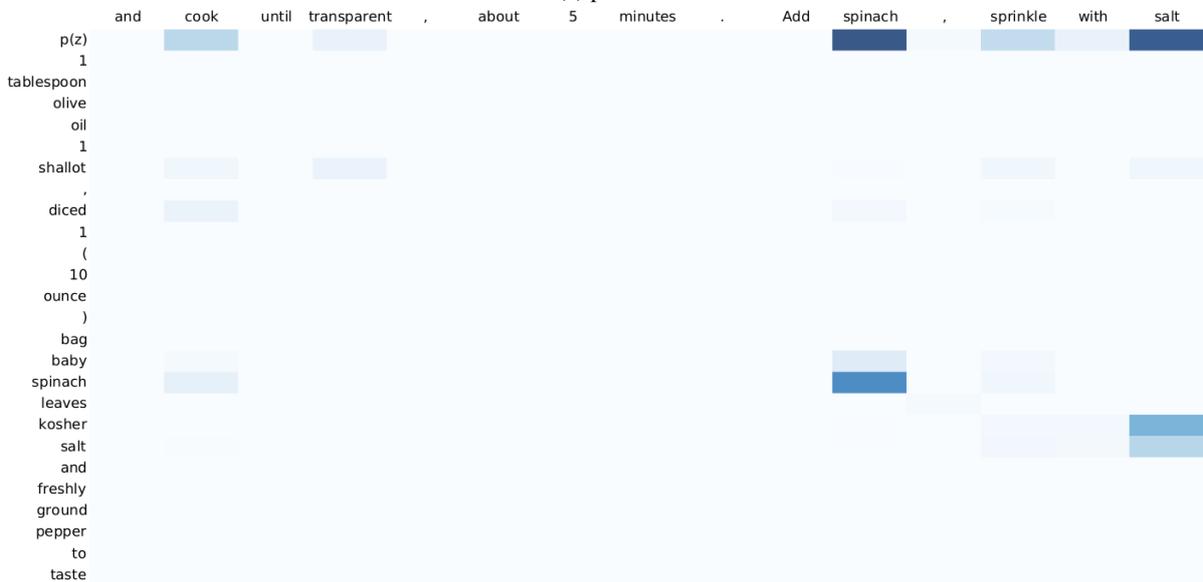

(b) part 2

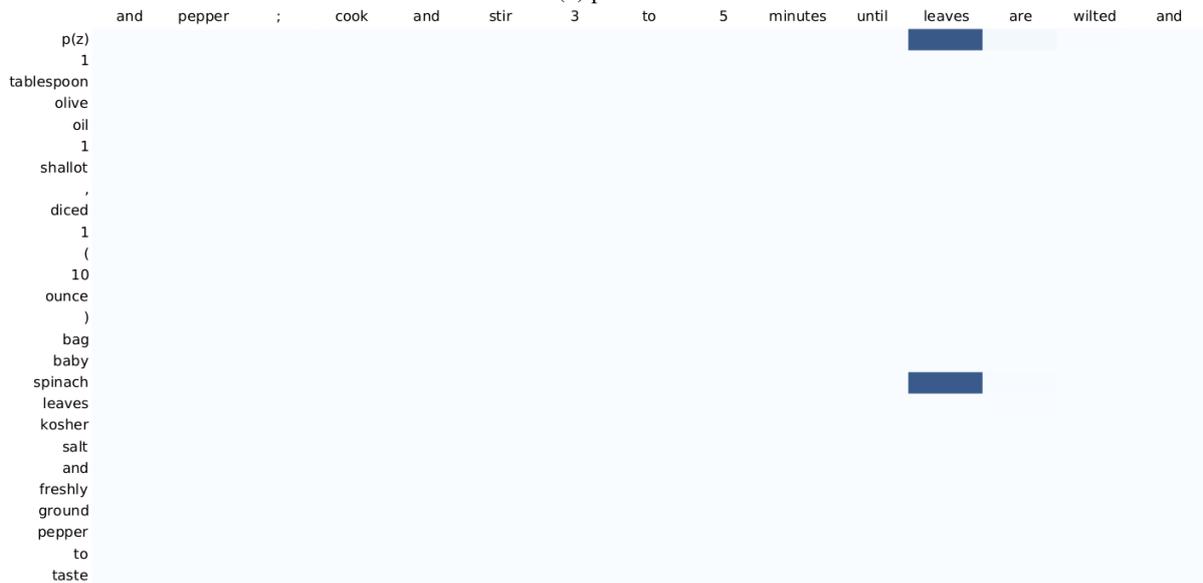

(c) part 3

Figure 7: Recipe heat map example 2.
